# Supplementary material for: SpecWatch: A Framework for Adversarial Spectrum Monitoring with Unknown Statistics
Source: arXiv:1710.05981 source file (2017-10-16)
Supplement: Supplementary file 1 [file appendix.tex]

%\appendices
\appendix
%\section{Proof of Lemma 1}
%\input{lemma1}
\section{}
\subsection{Proof of Lemma 2}~\label{lemma2 proof}
\input{lemma2}

%\section{Proof of Lemma 3}
%\input{lemma3}
%
%\section{Proof of Lemma 4}
%\input{lemma4}

\subsection{Proof of Lemma 5}\label{lemma5 proof}
\input{lemma5}

\subsection{Proof of Lemma 6}\label{lemma6 proof}
\input{lemma6}
